# Supplementary material for: PolyFootNet: Extracting Polygonal Building Footprints in Off-Nadir Remote Sensing Images
Source: arXiv:2408.08645 source file (2025-04-22)
Supplement: Supplementary file 1 [file Appendix.tex]

\section{Appendix Name}
\label{sec:Appendix_}

Here is content of the work appendix. In the general case there are more than one appendixes.
